# Supplementary material for: Dipole-dipole-interaction-induced entanglement between two-dimensional ferromagnets
Source: arXiv:2403.13354 source file (2024-03-20)
Supplement: Supplementary file 1 [file Supplemental_clean.pdf]

# Supplemental: Dipole-dipole-interaction-induced entanglement between two-dimensional ferromagnets

D. Wuhrer,[1,2] N. Rohling,[1] and W. Belzig[1,2]
[1)] *Fachbereich Physik, Universität Konstanz, D-78457 Konstanz, Germany*
[2)] *Authors to whom correspondence should be addressed: dennis.wuhrer@uni-konstanz.de and wolfgang.belzig@uni-konstanz.de*

(Dated: 4 March 2024)

## A. Classical ground state

In the Main part of this work we referred to the different phases of the classical ground state the system of two 2D FMs coupled by dipole interaction takes and here we will derive the different ground state configurations analytically. Starting from the Hamiltonian, Eqs. (1+6) in the main part,

$$\hat{H} = \hat{H}_A + \hat{H}_B + \hat{H}_{\text{int}}\,, \tag{S1}$$

we substitute each spin with its expectation value $\hat{\boldsymbol{S}}_i \to \boldsymbol{S}_i = \langle \hat{\boldsymbol{S}}_i \rangle$ and make the ansatz

$$\boldsymbol{S}_i = S \begin{pmatrix} \sin\left(\vartheta_{A/B}\right) \\ 0 \\ \cos\left(\vartheta_{A/B}\right) \end{pmatrix}\,, \qquad \boldsymbol{r}_i \in A/B \tag{S2}$$

for each spin belonging to FM $A$ or $B$. Here we already assumed that the ferromagnetic exchange interaction dominates inside each FM. The orientation of each spin is limited to the $x$-$z$-plane due to the anisotropies. The energy depending on the angles $\vartheta_A$ and $\vartheta_B$ is given by

$$E_{\text{cl}} = \text{const.} + \frac{NS^2}{2}\left\{-c_\Delta c_\Omega \tilde{A} + c_\Delta \Sigma D_{\boldsymbol{0}} - c_\Omega \delta D_{\boldsymbol{0}}\right\}\,. \tag{S3}$$

where we introduced $\Delta = \vartheta_A - \vartheta_B$, $\Omega = \vartheta_A + \vartheta_B$ and

$$\tilde{A} = 2S\left[K_z - (K_x + 3D_{x|\boldsymbol{0}})\right]\,, \qquad \Sigma D_{\boldsymbol{k}} = S\left[2D^{\text{int}}_{\boldsymbol{k}} - 3\left(D^{\text{int}}_{x|\boldsymbol{k}} + D^{\text{int}}_{z|\boldsymbol{k}}\right)\right]\,, \qquad \delta D_{\boldsymbol{k}} = 3S\left(D^{\text{int}}_{z|\boldsymbol{k}} - D^{\text{int}}_{x|\boldsymbol{k}}\right) \tag{S4}$$

with the definition of $D^{\text{int}}_{\alpha|\boldsymbol{k}}$ given in Sec. B.

The minimization of Eq. (S3) is now done with respect to $\Delta$ and $\Omega$ yielding

$$\frac{\partial \tilde{E}_{\text{cl}}}{\partial \Delta} = s_\Delta\left[c_\Omega \tilde{A} - \Sigma D_0\right] = 0\,, \qquad \frac{\partial \tilde{E}_{\text{cl}}}{\partial \Omega} = s_\Omega\left[c_\Delta \tilde{A} + \delta D_0\right] = 0\,, \tag{S5}$$

where we introduced $\tilde{E}_{\text{cl}} = E_{\text{cl}}/(NS^2)$. These equations have two possible solutions

$$\left(\cos(\Delta) = -\frac{\delta D_0}{\tilde{A}} \quad \wedge \quad \cos(\Omega) = \frac{\Sigma D_0}{\tilde{A}}\right) \qquad \vee \qquad \sin(\Delta) = 0 = \sin(\Omega)\,. \tag{S6}$$

To check whether or not they are minima of Eq. (S3) we calculate the Hessian, which is the matrix of second derivatives. The second derivatives of the energy are given by

$$\frac{\partial^2 \tilde{E}_{\text{cl}}}{\partial \Delta^2} = c_\Delta\left[c_\Omega \tilde{A} - \Sigma D_0\right]\,, \qquad \frac{\partial^2 \tilde{E}_{\text{cl}}}{\partial \Omega^2} = c_\Omega\left[c_\Delta \tilde{A} + \delta D_0\right]\,, \qquad \frac{\partial^2 \tilde{E}_{\text{cl}}}{\partial \Delta \partial \Omega} = -s_\Delta s_\Omega \tilde{A}\,. \tag{S7}$$

If we enter the first solution into the second derivatives this yields

$$\frac{\partial^2 \tilde{E}_{\text{cl}}}{\partial \Delta^2} = 0\,, \qquad \frac{\partial^2 \tilde{E}_{\text{cl}}}{\partial \Omega^2} = 0\,, \tag{S8}$$

which yields for the eigenvalues $\lambda_{1/2}$ of the Hessian

$$\lambda_{1/2} = \pm\left|\frac{\partial^2 \tilde{E}_{\text{cl}}}{\partial \Delta \partial \Omega}\right| \gtrless 0\,, \tag{S9}$$

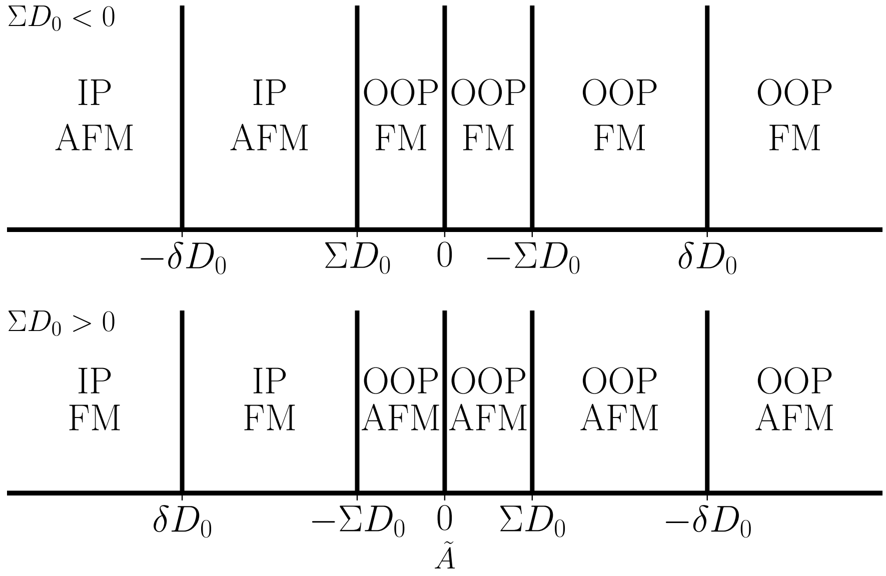


FIG. S1. Different orientations take from dipole-dipole interaction coupled 2D square lattice ferromagnets dependent on $\tilde{A}$. OOP (IP) stands for out of plane (in plane) and describes a configuration in which the magnetisation of both ferromagnets stands perpendicular to (lies in) the plane of the ferromagnet. FM (AFM) stands for a ferromagnetic (antiferromagnetic) ordering which means that the magnetisation of both ferromagnets is parallel (antiparallel) oriented with respect to each other.

which makes the Hessian indefinite and therefore this is no minima in the energy.

For the second solution, $\Delta,\Omega \in \{0,\pi\}$, we get for the derivatives

$$\frac{\partial^2 \tilde{E}_{\text{cl}}}{\partial \Delta^2} = r_\Delta \left[ r_\Omega \tilde{A} - \Sigma D_0 \right], \qquad \frac{\partial^2 \tilde{E}_{\text{cl}}}{\partial \Omega^2} = r_\Omega \left[ r_\Delta \tilde{A} + \delta D_0 \right], \qquad \frac{\partial^2 \tilde{E}_{\text{cl}}}{\partial \Delta \partial \Omega} = 0, \tag{S10}$$

where $r_\Delta, r_\Omega = +1$ for $\Omega,\Delta = 0$ and $-1$ for $\Omega,\Delta = \pi$. As the mixed derivative vanishes we need both pure derivatives to be larger than zero

$$r_\Delta \left[ r_\Omega \tilde{A} - \Sigma D_0 \right] > 0, \qquad r_\Omega \left[ r_\Delta \tilde{A} + \delta D_0 \right] > 0. \tag{S11}$$

For the system at hand, two 2D square lattice ferromagnets, the dipole sums $D^{\text{int}}_{x|0}$ and $D^{\text{int}}_{y|0}$ along the $x$ and $y$-direction are equal. This yields

$$\Sigma D^{\text{int}}_0 = 2D^{\text{int}}_0 - 3(D^{\text{int}}_{x|0} + D^{\text{int}}_{z|0}) = 2D^{\text{int}}_{y|0} - (D^{\text{int}}_{x|0} + D^{\text{int}}_{z|0}) = D^{\text{int}}_{x|0} - D^{\text{int}}_{z|0}, \tag{S12}$$

where we used

$$D^{\text{int}}_0 = \sum_{\delta} \frac{D^{\text{int}}}{|\delta|^3} = \sum_{\delta} \frac{D^{\text{int}}(\delta_x^2 + \delta_y^2 + \delta_z^2)}{|\delta|^5} = D^{\text{int}}_{x|0} + D^{\text{int}}_{y|0} + D^{\text{int}}_{z|0}. \tag{S13}$$

with the definition of $\delta D_0$ in Eq. (S4) we see that in this system $\delta D_0 = -3\Sigma D_0$. Therefore, condition Eq. (S11) depends only on the sign of $\Sigma D_0$ and the relation of $\tilde{A}$ and $\Sigma D_0$. From all possible minima in the energy we choose global minima, the one with the lowest energy. The different configurations taken depending on the sign of $\Sigma D_0$ and the value of $\tilde{A}$ are shown in Fig. S1.

The different combinations of $r_\Omega$ and $r_\Delta$ yield

$$r_\Omega = 1 = r_\Delta: \qquad \Omega = 0, \quad \Delta = 0, \qquad \vartheta_A = 0, \quad \vartheta_B = 0, \tag{S14}$$

$$r_\Omega = -1 = r_\Delta: \qquad \Omega = \pi, \quad \Delta = \pi, \qquad \vartheta_A = \pi, \quad \vartheta_B = 0, \tag{S15}$$

$$r_\Omega = 1 = -r_\Delta: \qquad \Omega = 0, \quad \Delta = \pi, \qquad \vartheta_A = \frac{\pi}{2}, \quad \vartheta_B = \frac{\pi}{2}, \tag{S16}$$

$$r_\Omega = -1 = -r_\Delta: \qquad \Omega = \pi, \quad \Delta = 0, \qquad \vartheta_A = \frac{\pi}{2}, \quad \vartheta_B = -\frac{\pi}{2}, \tag{S17}$$

or $\vartheta_A$ and $\vartheta_B$ interchanged.

### B. Dipole-Sums

The dipole-dipole interaction consists of two parts given by Eqs. (4+6) in the main part. The interaction strength for two spins at $\boldsymbol{r}_i$ and $\boldsymbol{r}_j$ is given in Eq. (5) in the main part as

$$D_{ij} = \frac{D}{\left|\boldsymbol{r}_i - \boldsymbol{r}_j\right|^3} = \frac{D}{|\boldsymbol{\delta}|^3}\,, \tag{S18}$$

where we introduced the connection vector $\boldsymbol{\delta} = \boldsymbol{r}_i - \boldsymbol{r}_j$ between both spins.

The second term in the dipole-dipole interaction contains elements of the unit vector along the connection line $\boldsymbol{e}_{ij} = \boldsymbol{\delta}/|\boldsymbol{\delta}|$. Therefore, the interaction strength coupling $\hat{S}_{i,\alpha}$ with $\hat{S}_{j,\beta}$, arising from the second term of the dipole-dipole interaction, is expressed in terms of the connection vector as

$$D_{\alpha\beta|ij} = D_{ij}\frac{\delta_\alpha\delta_\beta}{|\boldsymbol{\delta}|^2} = D\frac{\delta_\alpha\delta_\beta}{|\boldsymbol{\delta}|^5}\,, \qquad D_{\boldsymbol{k}} = \sum_{\boldsymbol{\delta}} \frac{D}{|\boldsymbol{\delta}|^3} e^{-i\boldsymbol{\delta}\cdot\boldsymbol{k}}\,, \qquad D_{\alpha\beta|\boldsymbol{k}} = \sum_{\boldsymbol{\delta}} \frac{D\delta_\alpha\delta_\beta}{|\boldsymbol{\delta}|^5} e^{-i\boldsymbol{\delta}\cdot\boldsymbol{k}} \tag{S19}$$

with $\alpha,\beta \in \{x,y,z\}$, $\delta_\alpha$ being the corresponding component of $\boldsymbol{\delta}$ and $\boldsymbol{\delta}$ running over all possible lattice sites with $\boldsymbol{\delta} \neq \boldsymbol{0}$.

If we regard the interaction between the FMs, then the $z$-components of $\boldsymbol{\delta}$ is always equal to the distance between both FMs, $l$, and the $x$ and $y$-component is allowed to be zero simultaneously.

For the 2D square lattice ferromagnets, all Fourier transformations of the dipole-dipole functions are real, except $D_{z\alpha|\boldsymbol{k}}$ with $\alpha \neq z$. Those are purely imaginary. Furthermore, for the uniform mode $\boldsymbol{k} = \boldsymbol{0}$ all terms $D_{\alpha\beta|0}$ with $\alpha \neq \beta$ vanish due to the symmetry of the system.

As we were not able to calculate $D_0^{\text{int}}$, $D_{x|0}^{\text{int}}$ and $D_{z|0}^{\text{int}}$ analytically nor numerically for an infinite system, we approximate those sums for the $\boldsymbol{k} = 0$ mode by an estimation of the remainder via an integral similar to the integral criteria for series. As we cope with a square lattice magnets we sum over all $\boldsymbol{\delta}$ with $\delta_x, \delta_y \in \{an | n \in \mathbb{Z}\}$, where $a$ is the lattice constant. Introducing $l' = l/a$ we define

$$S_1 = \sum_{n_x,n_y=-\infty}^{\infty} \frac{1}{\sqrt{n_x^2 + n_y^2 + l'^2}^{\,n}}\,, \qquad S_2 = \sum_{n_x,n_y=-\infty}^{\infty} \frac{n_x^2 + n_y^2}{\sqrt{n_x^2 + n_y^2 + l'^2}^{\,5}}\,. \tag{S20}$$

We split each sum in two parts. First $S_{\alpha,R}$ with $\rho^2(n_x,n_y) = n_x^2 + n_y^2 \leq R^2$ and second $\Delta S_{\alpha,R}$ with $\rho^2(n_x,n_y) > R^2$ for a radius $R \gg l'$. The second part we approximate by an integral similar to the integral criteria for one-dimensional sums over monotone decreasing function. As one can see from Eq. (S20), the arguments of both sums are rotational symmetric in the $n_x$-$n_y$-plane and decrease with increasing $\rho(n_x,n_y)$. Therefore, we will use polar coordinates to calculate the integrals. Then the estimates are given by

$$\Delta S_{1,R} \approx 2\pi \int_R^\infty \mathrm{d}\rho \frac{\rho}{\sqrt{\rho^2 + l'^2}^{\,n}} = \frac{2\pi}{n-2}\frac{1}{\sqrt{R^2 + l'^2}^{\,n-2}}\,, \tag{S21}$$

$$\Delta S_{2,R} \approx 2\pi \int_R^\infty \mathrm{d}\rho \frac{\rho^3}{\sqrt{\rho^2 + l'^2}^{\,5}} = \frac{\pi}{3}\frac{3R^2 + 2l'^2}{\sqrt{R^2 + l'^2}^{\,3}}\,. \tag{S22}$$

While the integral criteria is useful to estimate an upper and lower bound, both will converge towards the same value for large $R$.

We want to remark that the dipole sum containing only $n_x^2$ or $n_y^2$ in the denominator can be rewritten into the second sum in Eq. (S20) due to the lattice symmetry of the square lattice.

### C. Energies

We derive the energy dispersion of magnons populating the coupled system with the Hamiltonian

$$\hat{H} = \hat{H}_A + \hat{H}_B + \hat{H}_{\text{int}}\,. \tag{S23}$$

With eigensystems of the spins given in the main part in Eq. (8) and the corresponding spin components defined in the main part in Eqs. (9+10) this yields for the Hamiltonian in the Form

$$\hat{H}_A = \sum_{i,j\in A} \hat{\boldsymbol{S}}_i^\dagger \Xi_{A|ij} \hat{\boldsymbol{S}}_j\,, \qquad \hat{H}_{\text{int}} = \sum_{\substack{i\in A\\ j\in B}} \hat{\boldsymbol{S}}_i^\dagger \Xi_{\text{int}|ij} \hat{\boldsymbol{S}}_j\,, \tag{S24}$$

the coefficients

$$\Xi^{11}_{A|ij} = -J_{ij} - K_z s^2_{\vartheta_A} - K_x c^2_{\vartheta_A} + D^A_{ij} - 3D^A_{x|ij} c^2_{\vartheta_A}\,, \qquad \Xi^{12}_{A|ij} = -3D^A_{xy|ij} c_{\vartheta_A} = \Xi^{21}_{A|ij}\,, \tag{S25}$$

$$\Xi^{13}_{A|ij} = (K_z - K_x) c_{\vartheta_A} s_{\vartheta_A} - 3D^A_{x|ij} c_{\vartheta_A} s_{\vartheta_A} = \Xi^{31}_{A|ij}\,, \qquad \Xi^{22}_{A|ij} = -J_{ij} + D^A_{ij} - 3D^A_{y|ij}\,, \tag{S26}$$

$$\Xi^{23}_{A|ij} = -3D^A_{xy|ij} s_{\vartheta_A} = \Xi^{32}_{A|ij}\,, \qquad \Xi^{33}_{A|ij} = -J_{ij} - K_z c^2_{\vartheta_A} - K_x s^2_{\vartheta_A} + D^A_{ij} - 3D^A_{x|ij} s^2_{\vartheta_A}\,, \tag{S27}$$

with similar terms for $\hat{H}_B$.

As we did not include a magnetic field, we do not have any terms linear in the spin components. The interaction part of the Hamiltonian is given by

$$\Xi^{11}_{\mathrm{int}|ij} = D^{\mathrm{int}}_{ij}\left[c_{\vartheta_A} c_{\vartheta_B} + s_{\vartheta_A} s_{\vartheta_B}\right] - 3\left[D^{\mathrm{int}}_{x|ij} c_{\vartheta_A} c_{\vartheta_B} + D^{\mathrm{int}}_{z|ij} s_{\vartheta_A} s_{\vartheta_B} - D^{\mathrm{int}}_{xz|ij}\left(s_{\vartheta_A} c_{\vartheta_B} + c_{\vartheta_A} s_{\vartheta_B}\right)\right]\,, \tag{S28}$$

$$\Xi^{12}_{\mathrm{int}|ij} = -3\left[D^{\mathrm{int}}_{xy|ij} c_{\vartheta_A} - D^{\mathrm{int}}_{yz|ij} s_{\vartheta_A}\right]\,, \qquad \Xi^{21}_{\mathrm{int}|ij} = -3\left[D^{\mathrm{int}}_{xy|ij} c_{\vartheta_B} - D^{\mathrm{int}}_{yz|ij} s_{\vartheta_B}\right] \tag{S29}$$

$$\Xi^{13}_{\mathrm{int}|ij} = D^{\mathrm{int}}_{ij} c_{\vartheta_A} s_{\vartheta_B} - 3\left[D^{\mathrm{int}}_{x|ij} c_{\vartheta_A} s_{\vartheta_B} - D^{\mathrm{int}}_{z|ij} s_{\vartheta_A} c_{\vartheta_B} + D^{\mathrm{int}}_{xz|ij}\left(c_{\vartheta_A} c_{\vartheta_B} - s_{\vartheta_A} s_{\vartheta_B}\right)\right]\,, \tag{S30}$$

$$\Xi^{31}_{\mathrm{int}|ij} = D^{\mathrm{int}}_{ij} s_{\vartheta_A} c_{\vartheta_B} - 3\left[D^{\mathrm{int}}_{x|ij} s_{\vartheta_A} c_{\vartheta_B} - D^{\mathrm{int}}_{z|ij} c_{\vartheta_A} s_{\vartheta_B} + D^{\mathrm{int}}_{xz|ij}\left(c_{\vartheta_A} c_{\vartheta_B} - s_{\vartheta_A} s_{\vartheta_B}\right)\right]\,, \tag{S31}$$

$$\Xi^{22}_{\mathrm{int}|ij} = -3\left[D^{\mathrm{int}}_{xy|ij} c_{\vartheta_A} - D^{\mathrm{int}}_{yz|ij} s_{\vartheta_A}\right]\,, \tag{S32}$$

$$\Xi^{23}_{\mathrm{int}|ij} = -3\left[D^{\mathrm{int}}_{xy|ij} s_{\vartheta_B} + D^{\mathrm{int}}_{yz|ij} c_{\vartheta_B}\right]\,, \qquad \Xi^{32}_{\mathrm{int}|ij} = -3\left[D^{\mathrm{int}}_{xy|ij} s_{\vartheta_A} + D^{\mathrm{int}}_{yz|ij} c_{\vartheta_A}\right]\,, \tag{S33}$$

$$\Xi^{33}_{\mathrm{int}|ij} = D^{\mathrm{int}}_{ij}\left[c_{\vartheta_A} c_{\vartheta_B} + s_{\vartheta_A} s_{\vartheta_B}\right] - 3\left[D^{\mathrm{int}}_{x|ij} s_{\vartheta_A} s_{\vartheta_B} + D^{\mathrm{int}}_{z|ij} c_{\vartheta_A} c_{\vartheta_B} + D^{\mathrm{int}}_{xz|ij}\left(s_{\vartheta_A} c_{\vartheta_B} + c_{\vartheta_A} s_{\vartheta_B}\right)\right]\,. \tag{S34}$$

After performing the linearized Holstein–Primakoff transformation, Eqs. (9+10) in the main part, and the Fourier transformation, Eq. (11) in the main part, we get the linear spin wave Hamiltonian

$$\hat{H} = \sum_{\boldsymbol{k}\in\mathrm{BZ}^+} (\hat{a}^\dagger_{\boldsymbol{k}}, \hat{b}^\dagger_{\boldsymbol{k}}, \hat{a}_{-\boldsymbol{k}}, \hat{b}_{-\boldsymbol{k}}) \begin{pmatrix} E_{A,\boldsymbol{k}} & \mu^*_{1,\boldsymbol{k}} & 2\xi^*_{A,\boldsymbol{k}} & \mu^*_{2,\boldsymbol{k}} \\ \mu_{1,\boldsymbol{k}} & E_{B,\boldsymbol{k}} & \mu^*_{2,\boldsymbol{k}} & 2\xi^*_{B,\boldsymbol{k}} \\ 2\xi_{A,\boldsymbol{k}} & \mu_{2,\boldsymbol{k}} & E_{A,\boldsymbol{k}} & \mu_{1,\boldsymbol{k}} \\ \mu_{2,\boldsymbol{k}} & 2\xi_{B,\boldsymbol{k}} & \mu^*_{1,\boldsymbol{k}} & E_{B,\boldsymbol{k}} \end{pmatrix} \begin{pmatrix} \hat{a}_{\boldsymbol{k}} \\ \hat{b}_{\boldsymbol{k}} \\ \hat{a}^\dagger_{-\boldsymbol{k}} \\ \hat{b}^\dagger_{-\boldsymbol{k}} \end{pmatrix}\,, \tag{S35}$$

with the parameters

$$\begin{aligned} E_{A,\boldsymbol{k}} = S\big[&(2c^2_{\vartheta_A} - s^2_{\vartheta_A})K_z + (2s^2_{\vartheta_A} - c^2_{\vartheta_A})K_x + 3\left(2s^2_{\vartheta_A} D_{x|0} - c^2_{\vartheta_A} D_{x|\boldsymbol{k}} - D_{y|\boldsymbol{k}}\right) - \\ &-2(J_{\boldsymbol{k}} - J_0) + 2(D_{\boldsymbol{k}} - D_0)\big] + \frac{S}{2}\left(c_\Omega \delta D_0 - c_\Delta \Sigma D_0\right)\,, \end{aligned} \tag{S36}$$

$$\xi_{A,\boldsymbol{k}} = -\frac{S}{2}\left[K_z s^2_{\vartheta_A} + K_x c^2_{\vartheta_A} + 3\left(c^2_{\vartheta_A} D_{x|\boldsymbol{k}} - D_{y|\boldsymbol{k}}\right)\right]\,, \tag{S37}$$

$$\mu_{1,\boldsymbol{k}} = \frac{S}{2}\left[D^{\mathrm{int}}_{\boldsymbol{k}} + \frac{1}{2}\left(c_\Delta \Sigma D_{\boldsymbol{k}} + c_\Omega \delta D_{\boldsymbol{k}}\right)\right] - \frac{3S}{2}\left[D^{\mathrm{int}}_{y|\boldsymbol{k}} - s_\Omega D^{\mathrm{int}}_{xz|\boldsymbol{k}} + i\left(c_{\vartheta_A} - c_{\vartheta_B}\right) D^{\mathrm{int}}_{xy|\boldsymbol{k}} - i\left(s_{\vartheta_A} - s_{\vartheta_B}\right) D^{\mathrm{int}}_{zy|\boldsymbol{k}}\right]\,, \tag{S38}$$

$$\mu_{2,\boldsymbol{k}} = \frac{S}{2}\left[-D^{\mathrm{int}}_{\boldsymbol{k}} + \frac{1}{2}\left(c_\Delta \Sigma D_{\boldsymbol{k}} + c_\Omega \delta D_{\boldsymbol{k}}\right)\right] + \frac{3S}{2}\left[D^{\mathrm{int}}_{y|\boldsymbol{k}} + s_\Omega D^{\mathrm{int}}_{xz|\boldsymbol{k}} + i\left(c_{\vartheta_A} + c_{\vartheta_B}\right) D^{\mathrm{int}}_{xy|\boldsymbol{k}} - i\left(s_{\vartheta_A} + s_{\vartheta_B}\right) D^{\mathrm{int}}_{zy|\boldsymbol{k}}\right]\,. \tag{S39}$$

$E_{\alpha,\boldsymbol{k}}$ and $\xi_{\alpha,\boldsymbol{k}}$ are purely real, but $\mu_{1,\boldsymbol{k}}$ and $\mu_{2,\boldsymbol{k}}$ can be complex due to the terms $D^{\mathrm{int}}_{xz|\boldsymbol{k}}$ and $iD^{\mathrm{int}}_{xy|\boldsymbol{k}}$ which are purely imaginary. For the uniform mode $\boldsymbol{k} = \boldsymbol{0}$ of a 2D square lattice magnet those terms are given by

$$D^{\mathrm{int}}_{xy|0} = \sum_{n_x,n_y\in\mathbb{Z}} \frac{a^2 D^{\mathrm{int}} n_x n_y}{\sqrt{(an_x)^2 + (an_y)^2 + l^2}^5} = \sum_{n_x,n_y\in\mathbb{N}} \frac{a^2 D^{\mathrm{int}} (n_x - n_x)(n_y - n_y)}{\sqrt{(an_x)^2 + (an_y)^2 + l^2}^5} = 0\,, \tag{S40}$$

$$D^{\mathrm{int}}_{\alpha z|0} = \sum_{n_x,n_y\in\mathbb{Z}} \frac{-aD^{\mathrm{int}} n_\alpha l}{\sqrt{(an_x)^2 + (an_y)^2 + l^2}^5} = -2\sum_{n_x,n_y\in\mathbb{N}} \frac{aD^{\mathrm{int}} (n_\alpha - n_\alpha) l}{\sqrt{(an_x)^2 + (an_y)^2 + l^2}^5} = 0\,. \tag{S41}$$

Thus for the $\boldsymbol{k} = 0$ mode all parameters are real. We further see that for $\vartheta_A = \vartheta_B$ $\mu_{1,\boldsymbol{k}}$ is real for all wave vectors.

Writing the Hamiltonian in the form of Eq. (S35), the eigenproblem for the eigenenergies is given by

$$\underbrace{\begin{pmatrix} E_{A,\boldsymbol{k}} & \mu_{1,\boldsymbol{k}}^* & 2\xi_{A,\boldsymbol{k}}^* & \mu_{2,\boldsymbol{k}}^* \\ \mu_{1,\boldsymbol{k}} & E_{B,\boldsymbol{k}} & \mu_{2,\boldsymbol{k}}^* & 2\xi_{B,\boldsymbol{k}}^* \\ -2\xi_{A,\boldsymbol{k}} & -\mu_{2,\boldsymbol{k}} & -E_{A,\boldsymbol{k}} & -\mu_{1,\boldsymbol{k}} \\ -\mu_{2,\boldsymbol{k}} & -2\xi_{B,\boldsymbol{k}} & -\mu_{1,\boldsymbol{k}}^* & -E_{B,\boldsymbol{k}} \end{pmatrix}}_{\tilde{H}_{\boldsymbol{k}}} \mathscr{U}_{\boldsymbol{k}} = \mathscr{U}_{\boldsymbol{k}} \begin{pmatrix} \varepsilon_{\alpha,\boldsymbol{k}} & 0 & 0 & 0 \\ 0 & \varepsilon_{\beta,\boldsymbol{k}} & 0 & 0 \\ 0 & 0 & -\varepsilon_{\alpha,-\boldsymbol{k}} & 0 \\ 0 & 0 & 0 & -\varepsilon_{\beta,-\boldsymbol{k}} \end{pmatrix}, \tag{S42}$$

where the $i$-th column of the Bogoliubov matrix $\mathscr{U}_{\boldsymbol{k}}$ is the eigenvector of $\tilde{H}_{\boldsymbol{k}}$ with eigenvalues $\pm\varepsilon_{i,\pm\boldsymbol{k}}$ and $i \in \{\alpha,\beta\}$. This results in a fourth order equation for the energy eigenvalues $\varepsilon_{\boldsymbol{k}}$ given by

$$\varepsilon_{\boldsymbol{k}}^4 - \varepsilon_{\boldsymbol{k}}^2\left(\tilde{E}_{A,\boldsymbol{k}}^2 + \tilde{E}_{B,\boldsymbol{k}}^2\right) + \tilde{E}_{A,\boldsymbol{k}}^2\tilde{E}_{B,\boldsymbol{k}}^2 - \Sigma_{\boldsymbol{k}}^2 = 0, \tag{S43}$$

where we defined

$$\tilde{E}_{i,\boldsymbol{k}}^2 = E_{i,\boldsymbol{k}}^2 - 2|\xi_{i,\boldsymbol{k}}|^2 + |\mu_{1,\boldsymbol{k}}|^2 - |\mu_{2,\boldsymbol{k}}|^2, \tag{S44}$$

$$\Sigma_{\boldsymbol{k}}^2 = \left|\mu_{1,\boldsymbol{k}}(E_{A,\boldsymbol{k}}+E_{B,\boldsymbol{k}}) - \left(\mu_{2,\boldsymbol{k}}^*(2\xi_{A,\boldsymbol{k}}) + \mu_{2,\boldsymbol{k}}\left(2\xi_{B,\boldsymbol{k}}^*\right)\right)\right|^2 - \left|\mu_{2,\boldsymbol{k}}(E_{A,\boldsymbol{k}}-E_{B,\boldsymbol{k}}) - \left(\mu_{1,\boldsymbol{k}}^*(2\xi_{A,\boldsymbol{k}}) - \mu_{1,\boldsymbol{k}}(2\xi_{B,\boldsymbol{k}})\right)\right|^2. \tag{S45}$$

This yields for the energies

$$\varepsilon_{\alpha,\boldsymbol{k}} = \sqrt{\frac{1}{2}\left(\tilde{E}_{A,\boldsymbol{k}}^2 + \tilde{E}_{B,\boldsymbol{k}}^2 + \sqrt{\left(\tilde{E}_{A,\boldsymbol{k}}^2 - \tilde{E}_{B,\boldsymbol{k}}^2\right)^2 + 4\Sigma_{\boldsymbol{k}}^2}\right)}, \qquad \varepsilon_{\beta,\boldsymbol{k}} = \sqrt{\frac{1}{2}\left(\tilde{E}_{A,\boldsymbol{k}}^2 + \tilde{E}_{B,\boldsymbol{k}}^2 - \sqrt{\left(\tilde{E}_{A,\boldsymbol{k}}^2 - \tilde{E}_{B,\boldsymbol{k}}^2\right)^2 + 4\Sigma_{\boldsymbol{k}}^2}\right)}. \tag{S46}$$

As we cope with similar magnets which yields $\tilde{E}_{A,\boldsymbol{k}} = \tilde{E}_{B,\boldsymbol{k}} = \tilde{E}_{\boldsymbol{k}}$ and $\xi_{A,\boldsymbol{k}} = \xi_{B,\boldsymbol{k}} = \xi_{\boldsymbol{k}}$ and only two possible configurations (OOP FM and IP AFM) $\Sigma_{\boldsymbol{k}}^2$ simplifies to

$$\Sigma_{\boldsymbol{k}}^2 = \left|2\mu_{1,\boldsymbol{k}}E_{\boldsymbol{k}} - 2\xi_{\boldsymbol{k}}\left(\mu_{2,\boldsymbol{k}}^* + \mu_{2,\boldsymbol{k}}\right)\right|^2 \tag{S47}$$

and yields for the energies

$$\varepsilon_{\alpha/\beta,\boldsymbol{k}} = \sqrt{\tilde{E}_{\boldsymbol{k}} \pm \left|2\mu_{1,\boldsymbol{k}}E_{\boldsymbol{k}} - 2\xi_{\boldsymbol{k}}\left(\mu_{2,\boldsymbol{k}}^* + \mu_{2,\boldsymbol{k}}\right)\right|}, \tag{S48}$$

which can be written as

$$\varepsilon_{\alpha,\boldsymbol{k}} = \sqrt{|E_{\boldsymbol{k}} + \mu_{1,\boldsymbol{k}}|^2 - |\mu_{2,\boldsymbol{k}} + 2\xi_{\boldsymbol{k}}|^2}, \qquad \varepsilon_{\beta,\boldsymbol{k}} = \sqrt{|E_{\boldsymbol{k}} - \mu_{1,\boldsymbol{k}}|^2 - |\mu_{2,\boldsymbol{k}} - 2\xi_{\boldsymbol{k}}|^2}. \tag{S49}$$

In the case of only real parameters, the Bogoliubov parameters are calculated analytically. The elements of the matrix $U_{\boldsymbol{k}}$ are given by

$$u_{1,\boldsymbol{k}} = \sqrt{\frac{E_{\boldsymbol{k}} + \mu_{1,\boldsymbol{k}} + \varepsilon_{\alpha,\boldsymbol{k}}}{4\varepsilon_{\alpha,\boldsymbol{k}}}}, \qquad u_{2,\boldsymbol{k}} = -\sqrt{\frac{E_{\boldsymbol{k}} - \mu_{1,\boldsymbol{k}} + \varepsilon_{\beta,\boldsymbol{k}}}{4\varepsilon_{\beta,\boldsymbol{k}}}} \tag{S50}$$

$$u_{3,\boldsymbol{k}} = u_{1,\boldsymbol{k}}, \qquad u_{4,\boldsymbol{k}} = -u_{2,\boldsymbol{k}}, \tag{S51}$$

$$\tag{S52}$$

and the elements of $V_{\boldsymbol{k}}$ by

$$v_{1,\boldsymbol{k}} = -\mathrm{sign}\left(\mu_{2,\boldsymbol{k}} + 2\xi_{\boldsymbol{k}}\right)\sqrt{\frac{E_{\boldsymbol{k}} + \mu_{1,\boldsymbol{k}} - \varepsilon_{\alpha,\boldsymbol{k}}}{4\varepsilon_{\alpha,\boldsymbol{k}}}}, \qquad v_{3,\boldsymbol{k}} = v_{1,\boldsymbol{k}}, \tag{S53}$$

$$v_{2,\boldsymbol{k}} = -\mathrm{sign}\left(\mu_{2,\boldsymbol{k}} - 2\xi_{\boldsymbol{k}}\right)\sqrt{\frac{E_{\boldsymbol{k}} - \mu_{1,\boldsymbol{k}} - \varepsilon_{\beta,\boldsymbol{k}}}{4\varepsilon_{\beta,\boldsymbol{k}}}}, \qquad v_{4,\boldsymbol{k}} = -v_{2,\boldsymbol{k}}. \tag{S54}$$

### D. Squeezing Parameters

We will limit on the derivation of the squeezing parameters for real systems only, which means systems where the Bogoliubov parameters are real, as this is the case for the uniform magnon mode, $\boldsymbol{k}=0$, regarded in the main part.

Our goal is the representation of the Bogoliubov matrix Eq. (13) in terms of the squeezing parameters. To determine this connection we can either use the connection between the Bogoliubov matrix and the quantum representation of the squeezing operator Eq. (22) or we use that the Bogoliubov matrix itself is an element of $\mathrm{Sp}(4,\mathbb{R})$, the group of real symplectic matrices. The Bogoliubov matrix $\mathscr{U}_{\boldsymbol{k}}$ can be expressed in terms of squeezing parameters by

$$\mathscr{U}_{\boldsymbol{k}} = \exp\left(\sum_{i=1}^{10} \theta_{i,\boldsymbol{k}} \Phi_i\right), \tag{S55}$$

where $\Phi_i$ are the matrix representation of the quantum generator $\hat{\Phi}_{i,\boldsymbol{k}}$ and thus the generators of the corresponding algebra $\mathrm{sp}(4,\mathbb{R})$. The squeezing parameters $\theta_{i,\boldsymbol{k}}$ are purely real while the involved generators $\Phi_i$ can be either purely real or purely imaginary.

If we assume that the involved interactions are small then we can write the Bogoliubov matrix as

$$\mathscr{U}_{\boldsymbol{k}} = \mathbb{1} + \sum_{i=1}^{10} \theta_{i,\boldsymbol{k}} \Phi_i . \tag{S56}$$

As we limit on real systems we can exclude all generators[58] with purely imaginary elements. The generators left are given by

$$\Phi_1 = \begin{pmatrix} 0 & 0 & 1 & 0 \\ 0 & 0 & 0 & -1 \\ 1 & 0 & 0 & 0 \\ 0 & -1 & 0 & 0 \end{pmatrix}, \quad \Phi_2 = \begin{pmatrix} 0 & 0 & 1 & 0 \\ 0 & 0 & 0 & 1 \\ 1 & 0 & 0 & 0 \\ 0 & 1 & 0 & 0 \end{pmatrix}, \quad \Phi_3 = \begin{pmatrix} 0 & 1 & 0 & 0 \\ -1 & 0 & 0 & 0 \\ 0 & 0 & 0 & 1 \\ 0 & 0 & -1 & 0 \end{pmatrix}, \quad \Phi_4 = \begin{pmatrix} 0 & 0 & 0 & 1 \\ 0 & 0 & 1 & 0 \\ 0 & 1 & 0 & 0 \\ 1 & 0 & 0 & 0 \end{pmatrix}. \tag{S57}$$

$\Phi_2$ commutes with $\Phi_1, \Phi_3$ and $\Phi_4$ which in turn form a closed subalgebra of $\mathrm{sp}(4,\mathbb{R})$. With this the Bogoliubov matrix becomes

$$\mathscr{U}_{\boldsymbol{k}} = \exp\left(\theta_{2,\boldsymbol{k}} \Phi_2\right) \exp\left(\theta_{\boldsymbol{k}} \Phi_{\boldsymbol{k}}\right), \qquad \Phi_{\boldsymbol{k}} = \frac{\boldsymbol{\theta}_{\boldsymbol{k}} \cdot \boldsymbol{\Phi}}{\theta_{\boldsymbol{k}}}, \tag{S58}$$

with the vectors $\boldsymbol{\theta}_{\boldsymbol{k}} = (\theta_{3,\boldsymbol{k}}, \theta_{1,\boldsymbol{k}}, \theta_{4,\boldsymbol{k}})^\top$, $\boldsymbol{\Phi} = (\Phi_3, \Phi_1, \Phi_4)^\top$ and the length of $\boldsymbol{\theta}_{\boldsymbol{k}}$ under the metric $\eta = \mathrm{diag}(1,-1,-1)$

$$\theta_{\boldsymbol{k}} = \sqrt{\boldsymbol{\theta}_{\boldsymbol{k}}^\top \eta \boldsymbol{\theta}_{\boldsymbol{k}}} = \sqrt{(\theta_{3,\boldsymbol{k}})^2 - (\theta_{1,\boldsymbol{k}})^2 - (\theta_{4,\boldsymbol{k}})^2}. \tag{S59}$$

using this definition squaring $\Phi_2$ and $\Phi_{\boldsymbol{k}}$ yields

$$(\Phi_2)^2 = \mathbb{1}, \qquad (\Phi_{\boldsymbol{k}})^2 = -\mathbb{1}, \tag{S60}$$

which simplifies Eq. (S58)

$$\mathscr{U}_{\boldsymbol{k}} = \left(\cosh(\theta_{2,\boldsymbol{k}})\mathbb{1} + \sinh(\theta_{2,\boldsymbol{k}})\Phi_2\right)\left(\cos(\theta_{\boldsymbol{k}})\mathbb{1} + \sin(\theta_{\boldsymbol{k}}) \frac{\boldsymbol{\theta}_{\boldsymbol{k}} \cdot \boldsymbol{\Phi}}{\theta_{\boldsymbol{k}}}\right). \tag{S61}$$

Due to the negative multiple of the unit matrix when squaring $L_{\boldsymbol{k}}$ we end up with trigonometric functions governing the dependency of $\theta_{\boldsymbol{k}}$. As the definition of $\theta_{\boldsymbol{k}}$ is arbitrary one could as well use $\eta' = \mathrm{diag}(-1,1,1)$ yielding $\theta'_{\boldsymbol{k}} = i\theta_{\boldsymbol{k}}$ and leading to hyperbolic functions in Eq. (S61). We have chosen $\eta$ such that $\theta_{\boldsymbol{k}}$ is always real in our system due to $(\theta_{3,\mathbf{0}})^2 > (\theta_{1,\mathbf{0}})^2 + (\theta_{4,\mathbf{0}})^2$ for all distances.

From this each element of the Bogoliubov matrix in terms of squeezing operators is given by

$$u_{1,\boldsymbol{k}} = \cos(\theta_{\boldsymbol{k}})\cosh(\theta_{2,\boldsymbol{k}}) + \frac{\theta_{1,\boldsymbol{k}}}{\theta_{\boldsymbol{k}}}\sin(\theta_{\boldsymbol{k}})\sinh(\theta_{2,\boldsymbol{k}}), \qquad u_{2,\boldsymbol{k}} = \frac{\theta_{4,\boldsymbol{k}}}{\theta_{\boldsymbol{k}}}\sin(\theta_{\boldsymbol{k}})\sinh(\theta_{2,\boldsymbol{k}}) + \frac{\theta_{3,\boldsymbol{k}}}{\theta_{\boldsymbol{k}}}\sin(\theta_{\boldsymbol{k}})\cosh(\theta_{2,\boldsymbol{k}}), \tag{S62}$$

$$u_{3,\boldsymbol{k}} = \frac{\theta_{4,\boldsymbol{k}}}{\theta_{\boldsymbol{k}}}\sin(\theta_{\boldsymbol{k}})\sinh(\theta_{2,\boldsymbol{k}}) - \frac{\theta_{3,\boldsymbol{k}}}{\theta_{\boldsymbol{k}}}\sin(\theta_{\boldsymbol{k}})\cosh(\theta_{2,\boldsymbol{k}}), \qquad u_{4,\boldsymbol{k}} = \cos(\theta_{\boldsymbol{k}})\cosh(\theta_{2,\boldsymbol{k}}) - \frac{\theta_{1,\boldsymbol{k}}}{\theta_{\boldsymbol{k}}}\sin(\theta_{\boldsymbol{k}})\sinh(\theta_{2,\boldsymbol{k}}), \tag{S63}$$

$$v_{1,\boldsymbol{k}} = \cos(\theta_{\boldsymbol{k}})\sinh(\theta_{2,\boldsymbol{k}}) + \frac{\theta_{1,\boldsymbol{k}}}{\theta_{\boldsymbol{k}}}\sin(\theta_{\boldsymbol{k}})\cosh(\theta_{2,\boldsymbol{k}}), \qquad v_{2,\boldsymbol{k}} = \frac{\theta_{4,\boldsymbol{k}}}{\theta_{\boldsymbol{k}}}\sin(\theta_{\boldsymbol{k}})\cosh(\theta_{2,\boldsymbol{k}}) + \frac{\theta_{3,\boldsymbol{k}}}{\theta_{\boldsymbol{k}}}\sin(\theta_{\boldsymbol{k}})\sinh(\theta_{2,\boldsymbol{k}}), \tag{S64}$$

$$v_{3,\boldsymbol{k}} = \frac{\theta_{4,\boldsymbol{k}}}{\theta_{\boldsymbol{k}}}\sin(\theta_{\boldsymbol{k}})\cosh(\theta_{2,\boldsymbol{k}}) - \frac{\theta_{3,\boldsymbol{k}}}{\theta_{\boldsymbol{k}}}\sin(\theta_{\boldsymbol{k}})\sinh(\theta_{2,\boldsymbol{k}}), \qquad v_{4,\boldsymbol{k}} = \cos(\theta_{\boldsymbol{k}})\sinh(\theta_{2,\boldsymbol{k}}) - \frac{\theta_{1,\boldsymbol{k}}}{\theta_{\boldsymbol{k}}}\sin(\theta_{\boldsymbol{k}})\cosh(\theta_{2,\boldsymbol{k}}). \tag{S65}$$

As shown in the work of Colas et al[58] the squeezing operator is a quantum representation of the Bogoliubov transformation. Therefore, the involved squeezing parameters in Eq. (18) in the main part and (S55) coincide.

## I. CALCULATION OF ENTANGLEMENT

Here we sketch how we calculated the entanglement using the logarithmic negativity, Eq. (26) in the main part. For this we want to use Eq. (45) of Ref.[10] which yields for the lowest symplectic eigenvalue of the covariance matrix $\gamma'$

$$\eta^- = \frac{1}{\sqrt{2}}\sqrt{\Sigma\gamma' - \sqrt{(\Sigma\gamma')^2 - 4\det\gamma'}}\,, \tag{S66}$$

with

$$\Sigma\gamma' = \det V_1 + \det V_3 - 2\det V_2\,, \qquad \gamma'_R = \begin{pmatrix} V_1 & V_2 \\ V_2^\top & V_3 \end{pmatrix}. \tag{S67}$$

Here $\gamma'$ refers to the definition of the covariance matrix used in Ref.[10] where they ordered $\hat{\boldsymbol{R}}$ differently as $\hat{\boldsymbol{R}}' = (\hat{q}_A, \hat{p}_A, \hat{q}_B, \hat{p}_B)^\top$ which is connected to $\hat{\boldsymbol{R}}$ via the transformation

$$\hat{\boldsymbol{R}}' = \begin{pmatrix} 1 & 0 & 0 & 0 \\ 0 & 0 & 1 & 0 \\ 0 & 1 & 0 & 0 \\ 0 & 0 & 0 & 1 \end{pmatrix} \hat{\boldsymbol{R}} = M\hat{\boldsymbol{R}}. \tag{S68}$$

This yields for $\gamma'$

$$\gamma' = M\gamma M^\top\,, \tag{S69}$$

where $\gamma$ is given in Eq. (27) in the main part.

Putting Eq. (27) in the main part and Eq. (S69) together we get for $\gamma'_R$

$$\gamma'_R = \frac{1}{2}\begin{pmatrix} \gamma_1 & 0 & \gamma_3 & 0 \\ 0 & \gamma_2 & 0 & \gamma_4 \\ \gamma_3 & 0 & e^{4\theta_2}\gamma_2 & 0 \\ 0 & \gamma_4 & 0 & e^{-4\theta_2}\gamma_1 \end{pmatrix}, \tag{S70}$$

where $\theta_2$ is the corresponding squeezing parameter and

$$\gamma_{1/2} = e^{\pm 2\theta_2}\left[1 + 2\frac{\theta_{1,0}^2 + \theta_{4,0}^2}{(\theta_0)^2}\sin(\theta_0) \pm 2\left(\frac{\theta_{1,0}}{2\theta_0}\sin(2\theta_0) + \frac{\theta_{3,0}\theta_{4,0}}{(\theta_0)^2}\sin^2(\theta_0)\right)\right], \tag{S71}$$

$$\gamma_{3/4} = \pm 2 e^{\pm 2\theta_2}\left(\frac{\theta_{4,0}}{\theta_0}\sin(2\theta_0) - \frac{\theta_{3,0}\theta_{4,0}}{(\theta_0)^2}\sin^2(\theta_0)\right). \tag{S72}$$

This then yields

$$\begin{aligned}\gamma_1\gamma_2 &= \left(1 + 2\frac{\theta_{1,0}^2 + \theta_{4,0}^2}{(\theta_0)^2}\sin(\theta_0)\right)^2 - 2\left(\frac{\theta_{1,0}}{2\theta_0}\sin(2\theta_0) + \frac{\theta_{3,0}\theta_{4,0}}{(\theta_0)^2}\sin^2(\theta_0)\right)^2 = \\ &= 1 + 4\left(\frac{\theta_{4,0}}{\theta_0}\sin(2\theta_0) - \frac{\theta_{3,0}\theta_{4,0}}{(\theta_0)^2}\sin^2(\theta_0)\right)^2,\end{aligned} \tag{S73}$$

where we used $\theta_0^2 = \theta_{3,0}^2 - \theta_{1,0}^2 - \theta_{4,0}^2$ several times in the manipulation of $\gamma_1\gamma_2$. This yields

$$\Sigma\gamma'_R = \frac{1}{2}(\gamma_1\gamma_2 - \gamma_3\gamma_4) = \frac{1}{2} + 4\left(\frac{\theta_{4,0}}{\theta_0}\sin(2\theta_0) - \frac{\theta_{3,0}\theta_{4,0}}{(\theta_0)^2}\sin^2(\theta_0)\right)^2, \tag{S74}$$

The determinant of $\gamma'_R$ is given by

$$\begin{aligned}\det\gamma'_R = \det(V_1V_3 - V_2V_2^\top) &= \frac{1}{16}\det\left[\begin{pmatrix} e^{4\theta_{2,0}}\gamma_1\gamma_2 & 0 \\ 0 & e^{-4\theta_{2,0}}\gamma_1\gamma_2 \end{pmatrix} - \begin{pmatrix} \gamma_3^2 & 0 \\ 0 & \gamma_4^2 \end{pmatrix}\right] = \\ &= \frac{1}{16}\left(e^{4\theta_{2,0}}\gamma_1\gamma_2 - \gamma_3^2\right)\left(e^{-4\theta_{2,0}}\gamma_1\gamma_2 - \gamma_4^2\right) = \frac{1}{16}(\gamma_1\gamma_2 + \gamma_3\gamma_4) = \frac{1}{16},\end{aligned} \tag{S75}$$

where we used $\gamma_3 = -e^{4\theta_{2,0}}\gamma_4$. We define

$$\kappa = \left| \frac{\theta_{4,0}}{\theta_0} \sin(2\theta_0) - \frac{\theta_{3,0}\theta_{4,0}}{(\theta_0)^2} \sin^2(\theta_0) \right| , \tag{S76}$$

then Eq. (S74) and Eq. (S75) yield

$$\begin{aligned}
\Sigma\gamma'_R - \sqrt{(\Sigma\gamma'_R)^2 - 4\det\gamma'_R} &= \frac{1}{2} + 4\kappa^2 - \sqrt{\left(\frac{1}{2} + 4\kappa^2\right)^2 - \frac{1}{4}} = \frac{1}{2} + 4\kappa^2 - \sqrt{4\kappa^2(1+4\kappa^2)} = \\
&= \frac{1}{2}\left[\left(1+4\kappa^2\right) + 4\kappa^2 - 4\kappa\sqrt{1+4\kappa^2}\right] = \frac{1}{2}\left[2\kappa - \sqrt{1+4\kappa^2}\right]^2 ,
\end{aligned} \tag{S77}$$

and finally

$$\eta^- = \frac{1}{\sqrt{2}}\sqrt{\frac{1}{2}\left[2\kappa - \sqrt{1+4\kappa^2}\right]^2} = \frac{1}{2}\left|2\kappa - \sqrt{1+4\kappa^2}\right| , \tag{S78}$$

which coincides with Eq. (29) in the main part.
